# Supplementary material for: PRINCIPLES: Synthetic Strategy Memory for Proactive Dialogue Agents
Source: arXiv:2509.17459 source file (2025-09-22)
Supplement: Supplementary file 1 [file revision.tex]

\begin{figure*}[h]
    \centering
    \includegraphics[width=1\textwidth]{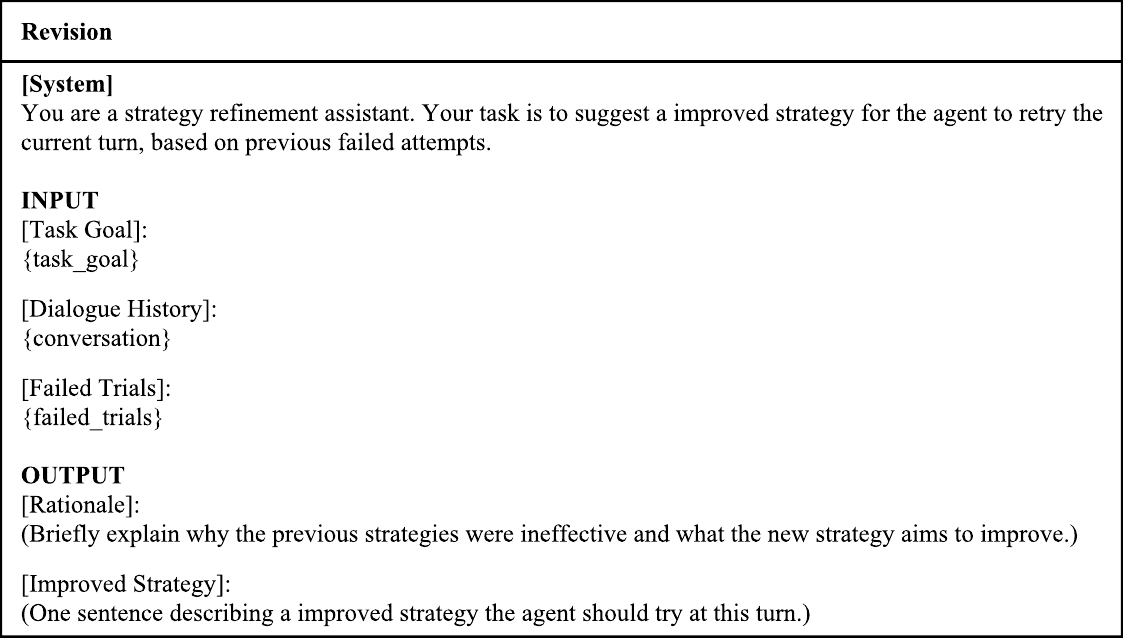}
    \caption{Prompt for revision module to revise the agent’s strategic decision.}
    \label{appendix:prompt:revision}
\end{figure*}
