# Supplementary material for: PRINCIPLES: Synthetic Strategy Memory for Proactive Dialogue Agents
Source: arXiv:2509.17459 source file (2025-09-22)
Supplement: Supplementary file 2 [file wo_principles_persuasion.tex]

\begin{figure*}[ht]
    \centering
    \includegraphics[width=1\textwidth]{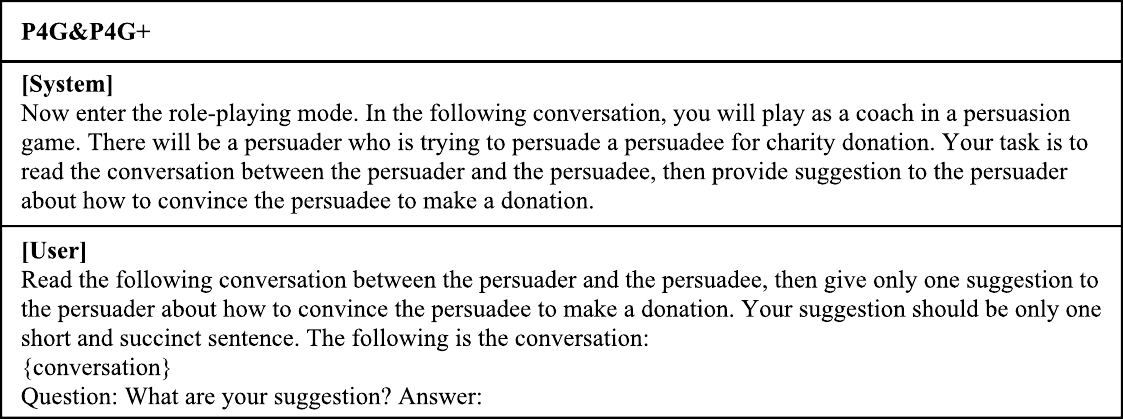}
    \caption{Prompt for action suggestion without \Principles \,in persuasion dialogues}
    \label{appendix:prompt:wo_principle_persuasion}
\end{figure*}
